# Supplementary material for: Dense Incremental Metric-Semantic Mapping for Multi-Agent Systems via Sparse Gaussian Process Regression
Source: arXiv:2103.16170 source file (2021-03-30)
Supplement: Supplementary file 1 [file Appendix.tex]

\section{Proof of Prop.~\ref{prop:gp_compression}}
\label{app:a}

Without loss of generality, assume $\mu_0(\bbx)=0$. The general result can be concluded by change of variables $f(\bbx)-\mu_0(\bbx)$. Let $X_*$ be an arbitrary finite set of query points, and $\bbf_*$ be the vector of evaluations of $f$ over $X_*$. To prove the posterior GPs are identical, regardless of which dataset is used for training, we will show that the Gaussian distribution of $\bbf_*$ conditioned on either dataset is the same. Let $\bff := f(X)$, $\hat\bbf=[\bbf^\top, \bbf_*^\top]^\top$, $\bbzeta=[y_{1,1},..., y_{n, m_n}]^\top$, and $D \in \mathbb{R}^{\sum_{j=1}^nm_j\times \sum_{j=1}^nm_j}$ be a diagonal matrix such that $D_{\sum_{k=0}^{i-1}m_k+j, \sum_{k=0}^{i-1}m_k+j}=\frac{1}{\sigma_i^2}$ for $j=1,...,m_i$. Our approach is to calculate $p(\bbf_*, \bbf | \bbzeta)$ from the joint distribution $p(\bbf_*, \bbf, \bbzeta)$ for the first dataset. Then, if we repeat the process for the second data set, calculating $p(\bbf_*, \bbf | \hat{\bbzeta})$, we end up with the same normal distribution. If the marginal of $\bbf_*$ is obtained by integrating out $\bbf$, the distributions $p(\bbf_*| \bbzeta)$, and $p(\bbf_*| \hat\bbzeta)$ remain the same. From conditional probability and since $\bbzeta$ depends on $\bbf$ only, we have $p(\bbf_*, \bbf, \bbzeta) = p(\bbzeta|\bbf)p(\bbf_*, \bbf)$. Let $\bbz=[ \bbzeta^\top, \hat\bbf^\top]^\top, \hat\bbz^\top=[ \hat\bbzeta^\top, \hat\bbf^\top]^\top$. The log likelihood of $\bfz$ is:  
\begin{equation}\label{logEq1}
\log p(\bbz) \propto \sum_{i=1}^n\sum_{j=1}^{m_i} -\frac{1}{2}\frac{(y_{i,j}-f(\bbx_i))^2}{\sigma_i^2}-\frac{1}{2} \hat\bbf^\top \bbOmega \hat\bbf,
\end{equation}
where $\begin{bmatrix} k_0(X,X) & k_0(X, X_*)\\ k_0(X_*, X)&k_0(X_*, X_*) \end{bmatrix}^{-1}=\begin{bmatrix}\bbOmega_{11} & \bbOmega_{12} \\ \bbOmega_{12}^{\top} & \bbOmega_{22}\end{bmatrix}=\bbOmega$. For the first dataset, let $\bbH$ be a matrix with elements ${\bbH}_{i, (\sum_{k=0}^{i-1}m_k+j)} = \frac{-1}{\sigma_i^2}$ for $i=1, \ldots, n$ and $j=1,\ldots, m_i$ with zero at the rest of its entries. Similarly, for the second dataset, let $\hat{\bbH}$ to be a matrix with elements ${\hat\bbH}_{i,i}=\frac{-m_i}{\sigma_i^2}$ for $i=1, ..., n$ and zero elsewhere. Rewrite \eqref{logEq1}:
\begin{align}
&\log p(\bbz) \propto -\frac{1}{2} \bbz^\top \bbOmega_{jnt} \bbz\label{logEq}\\
&\scaleMathLine{\bbOmega_{jnt} := \begin{bmatrix}D^{-1} & \bbH^\top & \bb0 \\ \bbH & \diag(\bbH\mathbf{1}) + \bbOmega_{11} & \bbOmega_{12}\\ \bb0 & \bbOmega_{12}^{\top} &\bbOmega_{22} \end{bmatrix} = \begin{bmatrix}D^{-1} & \bbG^\top \\ \bbG & \bbOmega_{cnd} \end{bmatrix},}\notag
%-\frac{1}{2} \bbz^\top  \begin{bmatrix}D^{-1} & \bbH^\top & \bb0 \\ \bbH & \diag(\bbH\mathbf{1}) & \bb0\\ \bb0 & \bb0 &\bb0 \end{bmatrix}\bbz \label{logEq}\\
%
%&\qquad \qquad\quad -\frac{1}{2} \bbz^\top  \begin{bmatrix}\bb0 & \bb0 & \bb0\\ \bb0 & \bbOmega_{11} & \bbOmega_{12} \\ \bb0 & \bbOmega_{12}^T & \bbOmega_{22}\end{bmatrix}\bbz = -\frac{1}{2} \bbz^\top \bbOmega_{jnt} \bbz,\notag
%
\end{align}
where $\mathbf{1}$ is a vector of ones.
% $\bbG:=[\bbH^\top , \bb0]^\top$, $\bbOmega_{cnd} := \begin{bmatrix} \bbOmega_{11}+\diag(\bbH\mathbf{1}) & \bbOmega_{12}\\ \bbOmega_{12}^\top & \bbOmega_{22} \end{bmatrix}$, and 
%where $\bbOmega_{jnt} := \begin{bmatrix}D^{-1} & \bbG^\top \\ \bbG & \bbOmega_{cnd} \end{bmatrix}$, $\bbG:=[\bbH^\top , \bb0]^\top$ in which we concatenate $|\bbf_*|$ zero rows to $\bbH$, $\bbOmega_{cnd} := \begin{bmatrix} \bbOmega_{11}+\diag(\bbH\mathbf{1}) & \bbOmega_{12}\\ \bbOmega_{12}^\top & \bbOmega_{22} \end{bmatrix}$, and $\mathbf{1}$ is an array with its entries to be all one.
%
This means $\bbz \sim \mathcal{N}(\bb0, \bbOmega_{jnt}^{-1})$, and hence $\hat\bbf| \bbzeta \sim \mathcal{N}(-\bbOmega_{cnd}^{-1}\bbG\bbzeta, \bbOmega_{cnd}^{-1})$. %\green{This step i.e. conditioning on some variable in multivariable normal distribution, its formula is famous I found it in the rasmussen and on the web, I think we can assume people can search it for themselves.}
Similarly for second dataset, define $\hat\bbOmega_{jnt} := \begin{bmatrix}\hat{D}^{-1} & \hat\bbG^\top \\ \hat\bbG & \hat\bbOmega_{cnd} \end{bmatrix}$, where $\hat\bbG:=[\hat\bbH^\top , \bb0]^\top$ and $\hat\bbOmega_{cnd}$ is defined by adding $\diag(\hat\bbH\mathbf{1})$ to the top left block of $\bfOmega$. Again, $\hat\bbz \sim \mathcal{N}(\bb0, \hat\bbOmega_{jnt}^{-1})$, so we can conclude $\hat\bbf| \hat\bbzeta \sim \mathcal{N}(-\hat\bbOmega_{cnd}^{-1}\hat\bbG\hat\bbzeta, \hat\bbOmega_{cnd}^{-1})$. The equivalence of the covariance matrices and means of these two normal distributions follows from $\hat\bbH\mathbf{1}=\bbH\mathbf{1}$ and $\hat\bbH\hat\bbzeta=\bbH\bbzeta$. \qed

%$\hat\bbG:=[\hat\bbH^\top , \bb0]^\top$ in which we concatenate $|X_*|$ zero rows to $\hat{\bbH}$, and $\hat\bbOmega_{cnd} := \begin{bmatrix} \bbOmega_{11}+\diag(\hat\bbH\mathbf{1}) & \bbOmega_{12}\\ \bbOmega_{12}^\top & \bbOmega_{22} \end{bmatrix}$. As before, we have $\hat\bbz \sim \mathcal{N}(\bb0, \hat\bbOmega_{jnt}^{-1})$, so we can conclude $\hat\bbf| \hat\bbzeta \sim \mathcal{N}(-\hat\bbOmega_{cnd}^{-1}\hat\bbG\hat\bbzeta, \hat\bbOmega_{cnd}^{-1})$. The equivalence of covariance matrices and means of these two normal distributions lies in the fact that $\hat\bbH\mathbf{1}=\bbH\mathbf{1}$, and $\hat\bbH\hat\bbzeta=\bbH\bbzeta$. \qed

% for first data set to be $n \times \sum_{i=1}^n m_i $ \green{$|\bbf|\times|\bbzeta|$} matrix, such that 
% $n \times n$ \green{$|\bbf|\times|\hat\bbzeta|$} matrix, such that

%===============================================================================%
\section{Proof of Prop.~\ref{prop:class_prediction}}
\label{app:b}
\noindent Let $l_c(z):=\mathbb{P}\prl{\argmin_\cls|f_\cls(\bfx)| = c \text{ and } \min_\cls |f_\cls(\bbx)| \leq |z|}$. Since $\mathbb{P}\prl{\min_\cls |f_\cls(\bbx)| \leq |z|}=\sum_\cls l_\cls(z)$:
\begin{equation*}
\scaleMathLine{\mathbb{P}\prl{\argmin_\cls|f_\cls(\bfx)| = c \;\bigg\vert\; \min_\cls |f_\cls(\bbx)| \leq |z|} =\frac{l_c(z)}{\sum_\cls l_\cls(z)}}
\end{equation*}
The term we are interested in computing is $\lim_{z \to 0} \frac{l_c(z)}{\sum_\cls l_\cls(z)}$. Let $\bfx$ be an arbitrary (test) point and define $\mu_\cls := \mu_{t,\cls}(\bfx)$ and $\sigma_\cls := \sigma_{t,\cls}(\bfx)$ for $\cls = 1,\ldots,N$. The GP prior of $f_\cls$ stipulates that its value at $\bfx$ has a density function $p(t) = \frac{1}{\sigma_\cls} \phi\big(\frac{t-\mu_\cls}{\sigma_\cls}\big)$. Hence, $\mathbb{P}(|f_\cls(\bbx)|\geq t) = 1-\Phi(\frac{|t|-\mu_\cls}{\sigma_\cls})+\Phi(\frac{-|t|-\mu_\cls}{\sigma_\cls})$. Note that $l_c(z)$ corresponds to the probability that $|f_c(\bbx)| \leq |f_\cls(\bbx)|$ for all $\cls$. Since all $f_\cls$ are independent of each other:
%\NA{Should there be $|t|$ here?}
\begin{equation*}
\scaleMathLine{l_c(z) = \int_{-z}^z \frac{\phi\big(\frac{t-\mu_c}{\sigma_c}\big)}{\sigma_c}\prod_{\cls\neq c}\biggl(1-\Phi\bigl(\frac{|t|-\mu_\cls}{\sigma_\cls}\bigr)+\Phi\bigl(\frac{-|t|-\mu_\cls}{\sigma_\cls}\bigr)\biggr)dt}
\end{equation*}
The claim is concluded by $\lim\limits_{z \to 0}\frac{l_c(z)}{2z}=\frac{1}{\sigma_c}\phi\big(\frac{-\mu_c}{\sigma_c}\big)$. \qed

%\NA{Is this expression correct?}

%Note the fact that $\mathbb{P}\prl{\argmin_i|f_i(\bfx)| = c \;\bigg\vert\; \min_i |f_i(\bbx)| = 0} = \lim\limits_{z \to 0} \mathbb{P}\prl{\argmin_i|f_i(\bfx)| = c \;\bigg\vert\; \min_i |f_i(\bbx)| \leq |z|}$ . Here we calculate $\mathbb{P}\prl{\argmin_i|f_i(\bfx)| = c \;\bigg\vert\; \min_i |f_i(\bbx)| \leq |z|}$, then limit $z\to 0$. Let $\scaleMathLine{l_c(z):=\mathbb{P}\prl{\argmin_i|f_i(\bfx)| = c \;\wedge\; \min_i |f_i(\bbx)| \leq |z|}}$, since $\mathbb{P}\prl{\min_i |f_i(\bbx)| \leq |z|}=\sum_i l_i(z)$ from conditional probability we can say:
%%
%\begin{equation*}
%\scaleMathLine{\mathbb{P}\prl{\argmin_i|f_i(\bfx)| = c \;\bigg\vert\; \min_i |f_i(\bbx)| \leq |z|} =\frac{l_c(z)}{\sum_i l_i(z)}}
%\end{equation*}
%%
%In order to calculate $l_c(z)$, note that it means the probability of the incident $f_c(\bbx_*) = t$ and for all $i\neq c$ we have $|f_i(\bbx_*)|\geq |t|$ such that $t \leq z$. Since $p(f_c(\bbx_*) = t) = \frac{1}{\sigma_c}\phi\big(\frac{t-\mu_c}{\sigma_c}\big)$, $\mathbb{P}(|f_i(\bbx_*)|\geq t) = 1-\Phi(\frac{|t|-\mu_i}{\sigma_i})+\Phi(\frac{-|t|-\mu_i}{\sigma_i})$, and since all $f_i$ are independent of each other we see:
%%
%\begin{equation*}
%l_c(z) = \int_{-z}^z \frac{\phi\big(\frac{t-\mu_c}{\sigma_c}\big)}{\sigma_c}\prod_{i\neq c}\big(1-\Phi(\frac{|t|-\mu_i}{\sigma_i})+\Phi(\frac{-|t|-\mu_i}{\sigma_i})\big)dt
%\end{equation*}
%%
%The claim is concluded from the fact that $\lim\limits_{z \to 0}\frac{l_c(z)}{2z}=\frac{1}{\sigma_c}\phi\big(\frac{-\mu_c}{\sigma_c}\big)$. \qed
